# Supplementary material for: Proofs and Programs about Open Terms
Source: arXiv:1805.07176 source file (2018-05-18)
Supplement: Supplementary file 1 [file paperformalization.tex]

\chapter[An On-paper Formalization]{An On-paper Formalization -- Type Preserving Compilation}

In his Dialectica Interpretation~\citep{Godel:58}, G\"odel develops an
interpretation of intuitionistic arithmetic into System-T, a system
intended to represent arithmetic with primitive recursion. We use a
stylized version of System-T, presented as a programming example. In
the following sections we show a presentation of System-T based on
that of \citet{Girard:1990}. In this example we think about System-T
as a rudimentary programming language with natural numbers and
recursion. We present a typical description of System-T as a formal
system, and prove some simple meta theorems. Finally, we show how it
is possible to translate System-T into Girard and Reynold's System-F.
This is intended to show how to specify a formal system, prove
properties about it and write computations that manipulate terms in
such a formal system. This is a simple example, but it is useful as a
somewhat complete example of how this kind of reasoning is done on
paper.

\section{System-T's Definition}

The syntax of the language:
\begin{displaymath}
  \begin{array}{rccll}
    \mbox{Types} & s, t & \bnfas & \stnat & \mbox{Natural numbers} \\
    & & & s \to t & \mbox{Functions} \\

    \mbox{Expressions} & e & \bnfas & \stz & \mbox{Zero} \\
    & & \bnfalt & \sts e & \mbox{Successor of a number} \\
    & & \bnfalt & \strec t e {e_z}{e_s} & \mbox{Recursion} \\
    & & \bnfalt & \stlam x s e & \mbox{Abstraction} \\
    & & \bnfalt & \app{e_1}{e_2} & \mbox{Application}\\
    & & \bnfalt & x & \mbox{Bound variable}\\
  \end{array}
\end{displaymath}

\subsection{The Type System}

The Typing context:
\begin{displaymath}
  \begin{array}{rccll}
    \mbox{Contexts} & \Gamma & \bnfas & \cdot & \mbox{Empty context} \\
    & & \bnfalt & \Gamma,x \oft t & \mbox{A typing assumption} \\
  \end{array}
\end{displaymath}

The typing:

% define contexts

\begin{displaymath}
  \begin{array}{c}
    \multicolumn{1}{l}
    {\boxed{\Gamma \vdash e \oft t}: \mbox{Expression $e$ is of type $t$ in context $\Gamma$.}} \vs

    \infer[\rl{t-z}]
    {\Gamma\vdash \stz \oft \stnat}
    {}

    \quad

    \infer[\rl{t-s}]
    {\Gamma\vdash \sts e \oft \stnat}
    {\Gamma\vdash e \oft \stnat}

    \vs

    \infer[\rl{t-rec}]
    {\Gamma\vdash \strec t e {e_z}{e_s} \oft t}
    {\Gamma\vdash e \oft \stnat
    & \Gamma\vdash e_z \oft t
    & \Gamma,f\oft t,x\oft \stnat\vdash e_s \oft t}

    \vs

    \infer[\rl{t-abs}]
    {\Gamma\vdash \stlam x s e \oft s \to t}
    {\Gamma, x \oft s\vdash e \oft t}

    \quad

    \infer[\rl{t-app}]
    {\Gamma\vdash \app{e_1}{e_2} \oft t}
    {\Gamma\vdash e_1\oft s \to t
    & \Gamma \vdash e_2 \oft s}

    \vs

    \infer[\rl{t-var}]
    {\Gamma \vdash x \oft t}
    {x\oft t \in \Gamma}
  \end{array}
\end{displaymath}

In order to be able to define an operational semantics that explains
how programs are to be evaluated we need to have a satisfactory
substitution operation. The definition of the operation is as follows:

\begin{displaymath}
  \begin{array}{r@{\ssub {e_y} y}lcl}
    & \stz & = & \stz \\
    & (\sts e) & = & \sts {(\ssub {e_y} y e)}\\
    & \strec t e {e_z}{e_s} & = &
      \strec t {\assub {e_y} y e} {\assub {e_y} y {e_z}}{\assub {e_y} y{e_s}} \\
    & & & \multicolumn{1}{l}{\quad\quad \mbox{when $y \neq f$ and $y \neq x$}}\\
    & \stlam x s e & = & \stlam x s {\assub {e_y} y e} \quad \mbox{when $y \neq x$}\\
    & \app {e_1}{e_2} & = & (\assub {e_y} y {e_1}) (\assub {e_y} y {e_2})\\
    & x & = & x \quad \mbox{when $y\neq x$}\\
    & y & = & e_y
  \end{array}
\end{displaymath}

An important property of the substitution operation is that typing
should be stable under substitution. The usual name for this theorem
is the Substitution Lemma.

\begin{thm}[Substitution lemma]
  \ \\If $\Gamma,y\oft s\vdash e \oft t$ and $\Gamma\vdash e_s \oft s$ then $\Gamma\vdash \assub {e_s} y e \oft t$.
\end{thm}

\begin{proof}
  \begin{flushleft}

  By structural induction on $e$:\\

    Case\ $e = \stz$: \\
    $\Gamma,y\oft s\vdash \stz\oft t$ \hfill Given\\
    $t = \stnat$ \hfill By inversion\\
    $\Gamma\vdash \stz \oft \stnat$ \hfill By \rl{t-z}
    \vs

    Case\ $e = \sts e'$: \hfill \\
    $\Gamma,y\oft s\vdash \sts e'\oft t$ \hfill Given\\
    $t = \stnat$ \hfill By inversion\\
    $\Gamma,y\oft s\vdash e'\oft \stnat$ \hfill By inversion\\
    $\Gamma\vdash \assub {e_s} y {e'} \oft \stnat$ \hfill By i.h.\\
    $\Gamma\vdash \sts{(\assub {e_s} y {e'})}\oft\stnat$ \hfill By \rl{t-s}\\
    $\Gamma\vdash \assub {e_s} y {(\sts e')}\oft\stnat$ \hfill By definition of substitution
    \vs

    Case\ $e = \strec t {e_r} {e_z}{e_s}$: \hfill \\
    $\Gamma,y\oft s\vdash\strec t {e_r} {e_z}{e_s}\oft t$ \hfill Given\\
    $\Gamma,y\oft s\vdash {e_r} \oft \stnat$ \hfill By inversion\\
    $\Gamma,y\oft s\vdash {e_z} \oft t$ \hfill By inversion\\
    $\Gamma,y\oft s, f\oft t,x\oft \stnat\vdash {e_s}\oft t$ \hfill By inversion\\
    $\Gamma\vdash \strec t {\assub {e_y} y e} {\assub {e_y} y {e_z}}{\assub {e_y} y{e_s}} \oft t$
    \hfill By i.h.\\
    $\Gamma\vdash \assub{e_y} y {(\strec t e {e_z}{e_s})} \oft t$ \hfill By definition of substitution
    \vs

    Case\ $e = \stlam x {t'} {e'}$: \\
    $\Gamma,y\oft s\vdash \stlam x {t'} {e'}\oft t$ \hfill Given\\
    $\Gamma,y\oft s\vdash \stlam x {t'} {e'}\oft t' \to t$ \hfill By inversion\\
    $\Gamma,y\oft s, x \oft t'\vdash e'\oft t$ \hfill By inversion\\
    $\Gamma,x \oft t'\vdash \assub{e_y} y {e'}\oft t$ \hfill By i.h.\\
    $\Gamma\vdash \stlam x {t'} (\assub{e_y} y {e'})\oft t' \to t$ \hfill By \rl{t-abs}\\
    $\Gamma\vdash \assub{e_y} y {(\stlam x {t'} {e'})}\oft t' \to t$ \hfill By definition of substitution
    \vs

    Case\ $e = \app{e_1}{e_2}$: \\
    $\Gamma,y\oft s\vdash \app{e_1}{e_2} \oft t$ \hfill Given\\
    $\Gamma,y\oft s\vdash e_1 \oft t' \to t$ \hfill By inversion\\
    $\Gamma,y\oft s\vdash e_2 \oft t'$ \hfill By inversion\\
    $\Gamma\vdash \assub{e_y} y {e_1} \oft t' \to t$ \hfill By i.h.\\
    $\Gamma\vdash \assub{e_y} y {e_2} \oft t'$ \hfill By i.h.\\
    $\Gamma\vdash \app {(\assub{e_y} y {e_1})} {(\assub{e_y} y {e_2})} \oft t$ \hfill By \rl{t-app}\\
    $\Gamma\vdash \assub{e_y} y {(\app{e_1}{e_2})} \oft t$ \hfill By definition of substitution
    \vs

    Case\ $e = y$: \\
    $\Gamma,y\oft s\vdash y\oft t$ \hfill Given\\
    $s = t$ \hfill By inversion and context lookup\\
    $\Gamma\vdash e_s \oft s$ \hfill Given\\
    $\Gamma\vdash \assub{e_y} y y$ \hfill Since $\assub{e_y} y y = e_y$\\
    $\Gamma\vdash e_s \oft s$ \hfill By definition of substutition
    \vs

    Case\ $e = x$ when $x\neq y$: \\
    $\Gamma,y\oft s\vdash x\oft t$ \hfill Given\\
    $\Gamma(x) = t$ \hfill by inversion and the fact that $x\neq y$\\
    $\Gamma\vdash x \oft t$ \hfill by \rl{t-var}

  \end{flushleft}
\end{proof}

%%% TODO binders need to satisify provisos

This is a simple proof done of in a somewhat detailed way. However, it
is not by any means, the most detailed proof one could have, as we
have glossed over details such as structural properties of the context
(e.g. weakening, contraction, and exchange). That a fully detailed
proof would have to show. The point of this proof is to show how a
moderately detailed proof requires a fair amount of DETAIL? and that
if we intend to mechanize and fully formalize such a proof all this
detail becomes important. The question that one should pose oneself
is: What would a good meta-language to represent this style of proof
on a computer?

\subsection{Operational Semantics}

\begin{displaymath}
  \begin{array}{c}
    \multicolumn{1}{l}
    {\boxed{e \isval}: \mbox{Expression $e$ is a value.}} \vs

    \infer
    {\stz \isval}{}

    \quad

    \infer
    {\sts e \isval}{}

    \quad

    \infer
    {\stlam x s e \isval}{}

    \vs

    \multicolumn{1}{l}
    {\boxed{e \stepsto e'}: \mbox{Expression $e$ steps to $e'$.}} \vs

    \infer
    {\app{e_1}{e_2} \stepsto \app{e'_1}{e_2}}
    {e_1 \stepsto e'_1}

    \quad

    \infer
    {\app {(\stlam x s e)} {e'} \stepsto \assub {e'} x e}
    {}

    \vs

    \infer
    {\strec t e {e_z}{e_s} \stepsto \strec t {e'} {e_z}{e_s}}
    {e \stepsto e'}

    \quad

    \infer
    {\strec t \stz {e_z}{e_s} \stepsto e_z}
    {}

    \vs

    \infer
    {\strec t {(\sts e)} {e_z}{e_s} \stepsto \assub {\strec t e {e_z}{e_s}} f {\assub e x {e_s}}}
    {}

  \end{array}
\end{displaymath}

So ...

\begin{thm}[Subject reduction]
  \ \\If $\mathcal{D}: \Gamma\vdash e \oft t$ and $\mathcal{E}: e \stepsto e'$ then $\Gamma\vdash e' \oft t$.
\end{thm}

\begin{proof}
  \begin{flushleft}

  by induction on $\mathcal{E}$ and inversion on $\mathcal{D}$\\

    Case $\mathcal{E}= \infer
    {\app {(\stlam x s e)} {e'} \stepsto \assub {e'} x e} {}$\\
    $\Gamma\vdash \app {(\stlam x s e)} {e'} \oft t$ \hfill Given\\
    $\Gamma\vdash \stlam x s e \oft s \to t$ \hfill By inversion on \rl{t-app}\\
    $\Gamma\vdash e' \oft s$ \hfill By inversion on \rl{t-app}\\
    $\Gamma,x\oft s\vdash e \oft t$ \hfill By inversion on \rl{t-abs}\\
    $\Gamma\vdash \assub {e'} x e \oft t$ \hfill By substitution lemma
    \vs

    Case $\mathcal{E}= \infer
      {\app{e_1}{e_2} \stepsto \app{e'_1}{e_2}}
      {e_1 \stepsto e'_1}$\\
    $\Gamma\vdash\app{e_1}{e_2}\oft t$ \hfill Given\\
    $\Gamma\vdash e_1\oft s \to t$ \hfill By inversion on \rl{t-app}\\
    $\Gamma\vdash e_2\oft s$ \hfill By inversion on \rl{t-app}\\
    $\Gamma\vdash e'_1\oft s \to t$ \hfill By i.h.\\
    $\Gamma\vdash \app{e'_1}{e_2}\oft t$ \hfill By rule \rl{t-app}
    \vs

    Case $\mathcal{E}= \infer
      {\strec t e {e_z}{e_s} \stepsto \strec t {e'} {e_z}{e_s}}
      {e \stepsto e'}$\\
    By a similar argument as the application case
    \vs

    Case $\mathcal{E}= \infer
      {\strec t \stz {e_z}{e_s} \stepsto e_z}{}$\\
    $\Gamma\vdash\strec t \stz {e_z}{e_s} \oft t$ \hfill Given\\
    $\Gamma\vdash e_z \oft t$ \hfill By inversion
    \vs

      Case $\mathcal{E}= \infer
      {\strec t {(\sts e)} {e_z}{e_s} \stepsto \assub {\strec t e {e_z}{e_s}} f {\assub e x {e_s}}}{}$\\
    $\Gamma\vdash\strec t {(\sts e)} {e_z}{e_s}\oft t$ \hfill Given\\
    $\Gamma\vdash e \oft \stnat$ \hfill By inversion on \rl{t-rec} and \rl{t-s}\\
    $\Gamma,f\oft t, x\oft nat \vdash e_s \oft t$ \hfill By inversion on \rl{t-rec}\\
    $\Gamma\vdash\assub {\strec t e {e_z}{e_s}} f {\assub e x {e_s}}\oft t$ \hfill By substitution lemma
    \vs
  \end{flushleft}
\end{proof}

At this point we have a definition of the source language, and we have
proven some nice properties of our language. To finish this example
lets consider a transformation of this language. A typical program
transformation is compiling a language into another. For this example
we will compile System-T to System-F that we introduce next.

\section{System-F}

The syntax of the language:
\begin{displaymath}
  \begin{array}{rccll}
    \mbox{Types} & S, T & \bnfas & \alpha & \mbox{Type Variables} \\
    & & & \sfall \alpha T & \mbox{Type quantifier} \\
    & & & S \to T & \mbox{Functions} \\

    \mbox{Expressions} & E & \bnfas & \sfLam \alpha E & \mbox{Type abstraction}\\
    & & & \sftapp{E}{T} & \mbox{Type application}\\
    & & & \sflam x s E & \mbox{Abstraction} \\
    & & & \app{E_1}{E_2} & \mbox{Application}\\
    & & & x & \mbox{Bound variable}\\
  \end{array}
\end{displaymath}

This language is much more expressive than System-T, and thus we can
use it as a target compilation for the language that we just defined.

\subsection{Typing and Operational Semantics}

The Typing context:
\begin{displaymath}
  \begin{array}{rccll}
    \mbox{Contexts} & \Delta & \bnfas & \cdot & \mbox{Empty context} \\
    & & \bnfalt & \Delta,x \oft T & \mbox{A typing assumption} \\
    & & \bnfalt & \Delta,\alpha & \mbox{A type assumption} \\
  \end{array}
\end{displaymath}

The typing:

% define contexts

\begin{displaymath}
  \begin{array}{c}
    \multicolumn{1}{l}
    {\boxed{\Delta \vdash T \istype}: \mbox{$T$ is a type in context $\Delta$.}} \vs

    \infer
    {\Delta\vdash \alpha\istype}
    {\alpha \in \Delta}

    \quad

    \infer
    {\Delta\vdash S \to T \istype}
    {\Delta\vdash S \istype & \Delta\vdash T \istype}

    \quad

    \infer
    {\Delta\vdash \sfall \alpha T \istype}
    {\Delta,\alpha\vdash T \istype}

    \vs

    \multicolumn{1}{l}
    {\boxed{\Delta \vdash E \oft T}: \mbox{Expression $E$ is of type $T$ in context $\Delta$.}} \vs

    \infer[\rl{T-tabs}]
    {\Delta\vdash \sfLam \alpha E \oft \sfall \alpha T}
    {\Delta,\alpha\vdash E \oft T}

    \quad

    \infer[\rl{T-tapp}]
    {\Delta\vdash \sftapp E S\oft \assub S \alpha T}
    {\Delta\vdash E\oft \sfall \alpha T & \Delta\vdash S \istype}

    \vs

    \infer[\rl{T-abs}]
    {\Delta\vdash \sflam x S E\oft S \to T}
    {\Delta, x \oft S\vdash E \oft T}

    \quad

    \infer[\rl{T-app}]
    {\Delta\vdash \app{E_1}{E_2} \oft T}
    {\Delta\vdash E_1\oft S \to T
    & \Delta \vdash E_2 \oft S}

    \vs

    \infer[\rl{T-var}]
    {\Delta\vdash x\oft T}
    {x \oft T \in \Delta}

  \end{array}
\end{displaymath}

We assume that when type-checking, we check against a well formed
type.

%TODO define substitution

\subsubsection{Operational Semantics}

\begin{displaymath}
  \begin{array}{c}
    \multicolumn{1}{l}
    {\boxed{E \isval}: \mbox{Expression $E$ is a value.}} \vs

    \infer
    {\sflam x S E \isval}
    {}

    \quad

    \infer
    {\sfLam \alpha E \isval}
    {}

    \vs

    \multicolumn{1}{l}
    {\boxed{E \stepsto E'}: \mbox{Expression $E$ steps to $E'$.}} \vs

    \infer
    {\app{E_1}{E_2} \stepsto \app{E'_1}{E_2}}
    {E_1 \stepsto E'_1}

    \quad

    \infer
    {\app {(\sflam x S E)} {E'} \stepsto \assub {E'} x E}
    {}

    \vs

    \infer
    {\sftapp{E} T \stepsto \sftapp{E'}{T}}
    {E \stepsto E'}

    \quad

    \infer
    {\sftapp {(\sfLam \alpha E)} {T} \stepsto \assub {T} \alpha E}
    {}

    \vs
  \end{array}
\end{displaymath}

Substitution operations:

\begin{displaymath}
  \begin{array}{r@{\ssub {T_\beta} \beta}lcl}
    & \sfall \alpha T & = & \sfall \alpha {(\assub {T_\beta} \beta T)} \quad \mbox{when $\alpha\neq\beta$} \\
    & S \to T & = & {(\assub {T_\beta} \beta S)} \to  {(\assub {T_\beta} \beta T)} \\
    & \alpha & = & \alpha \quad \mbox{when $\alpha\neq\beta$}\\
    & \beta & = & T_\beta
  \end{array}
\end{displaymath}

\begin{displaymath}
  \begin{array}{r@{\ssub {T_\beta} \beta}lcl}
    & \sfLam \alpha E & = & \sfLam \alpha {(\assub {T_\beta} \beta E)} \quad \mbox{when $\alpha\neq\beta$}\\
    & \sftapp {E}{S} & = & \sftapp {(\assub {T_\beta} \beta {E})} {\assub {T_\beta} \beta {S}}\\
    & \sflam x S E & = & \sflam x {(\assub {T_\beta} \beta S)} {(\assub {T_\beta} \beta E)}\\
    & \app {E_1}{E_2} & = & (\assub {T_\beta} \beta {E_1}) (\assub {T_\beta} \beta {E_2})\\
    & x & = & x\\
  \end{array}
\end{displaymath}

\begin{displaymath}
  \begin{array}{r@{\ssub {E_y} y}lcl}
    & \sfLam \alpha E & = & \sfLam \alpha {(\assub {E_y} y E)}\\
    & \sftapp {E}{S} & = & \sftapp {(\assub {E_y} y {E})} {S}\\
    & \sflam x S E & = & \sflam x S {(\assub {E_y} \beta E)} \quad \mbox{when $x \neq y$}\\
    & \app {E_1}{E_2} & = & (\assub {E_y} y {E_1}) (\assub {E_y} y {E_2})\\
    & x & = & x \quad \mbox{when $x \neq y$}\\
    & y & = & E_y\\
  \end{array}
\end{displaymath}

Lemmata:

\begin{thm}[Substitution lemma for types and terms]
  \ \\If $\mathcal{D}: \Gamma\vdash S \istype$ and $\mathcal{E}:\Gamma,\alpha\vdash T \istype$
  then $\Gamma\vdash \assub S \alpha T\istype$.
  \ \\If $\mathcal{D}: \Gamma\vdash S \istype$ and $\mathcal{E}:\Gamma,\alpha\vdash E\oft T$
  then $\Gamma\vdash \assub S \alpha E \oft \assub S \alpha T$.
  \ \\If $\mathcal{D}: \Gamma\vdash E_S \oft S$ and $\mathcal{E}:\Gamma,x\oft S\vdash E\oft T$
  then $\Gamma\vdash \assub {E_S} x E \oft T$.
\end{thm}

\begin{proof}
The first lemma is proved by induction on the structure of $T$.\\
The second lemma is proved by induction on the structure of $E$ and uses the previous lemma.\\
The third is proved by induction on the structure of $E$.\\
\end{proof}

\subsection{Using System-F}

It is not obvious how to represent usual programming concepts in pure
System-F. However the system is very expressive. Here, I discuss just
a hint of what is possible. The idea is to introduce enough
constructions here to make the compilation of System-T to System-F (in Section: \ref{sec:compTtoF})
straightforward.

\subsubsection*{Products}

It is a good idea to gather inspiration from Church encodings in the
untyped $\lambda$-calculus and adapt them to System-F. For example, in
the untyped $\lambda$-calculus pairs (or products) are represented
with the following terms:

\begin{displaymath}
  \begin{array}{rcl}
    (x, t) & := & \sflam f {} {\app {\app f x} y}\\
    \app{\code{fst}} p & := & \app p {(\sflam x {} {\sflam y {} x})}\\
    \app{\code{snd}} p & := & \app p {(\sflam x {} {\sflam y {} y})}\\
  \end{array}
\end{displaymath}

In this encoding pairs are represented as a higher-order function that
takes a selector function (variable $f$) that will choose the
appropriate element of the pair. In consequence, both projections are
exactly the functions that select either the first or the second
element of the pair.

Simply typed systems like System-T lack the power to represent pairs
this way as abstraction over types is really necessary. The System-F
versions follow the untyped versions but appropriately add
quantification over types.

\begin{displaymath}
  \begin{array}{rcl}
    \sfprod \alpha \beta & := & \sfall \gamma {(\alpha \to \beta \to \gamma) \to \gamma}\\
    \sfpair \  \  & : & \sfall \alpha \sfall \beta \alpha \to \beta \to \sfprod \alpha \beta\\
    \sfpair {E_1^\alpha} {E_2^\beta} & = & \sfLam \gamma {\sflam f {\alpha\to\beta\to\gamma} {\app {\app f {E_1}} {E_2}}}\\
    \sffst {} & : & \sfprod \alpha \beta \to \alpha\\
    \sffst E & = & \app {\sftapp E \alpha} {(\sflam x {\alpha} {\sflam y {\beta} x})}\\
    \sfsnd {} & : & \sfprod \alpha \beta \to \beta\\
    \sfsnd E & = & \app {\sftapp E \beta} {(\sflam x {\alpha} {\sflam y {\beta} y})}\\
  \end{array}
\end{displaymath}

% TODO explain

\subsubsection*{Representing Natural Numbers}

To represent natural numbers in System-F, one uses the idea of
representing a number by iterative application of a function.

\begin{displaymath}
  \begin{array}{rcl}
    \sfnat & = & \sfall \alpha \alpha \to (\alpha \to \alpha) \to \alpha\\
    \sfz & : & \sfnat\\
    \sfz & = & \sfLam \alpha {\sflam z \alpha {\sflam f {\alpha\to\alpha} z}}\\
    \sfs \ & : & \sfnat \to \sfnat \\
    \sfs E & = & \sfLam \alpha {\sflam z \alpha {\sflam f {\alpha\to\alpha} {\app f {(\app{\app {\sftapp E {\alpha}} z} f)}}}}
  \end{array}
\end{displaymath}

An interesting aspect of this is how much, the type of natural numbers
looks like the induction principle for natural
numbers. %Expand and explain better
However, if we want System-T style recursion we need access to the
predecessor, this requires keeping track of it during the
iteration/induction.

\begin{displaymath}
  \begin{array}{rcll}
    \underline{\code{rec}} & : & \multicolumn{2}{l}{ \sfall \alpha \sfnat \to \alpha \to (\sfprod \sfnat \alpha \to \alpha) \to \alpha} \\
    \sfrec \alpha E {E_z} {E_s} & = & \sffst (E & \sftapp{} {\sfprod {\alpha} \sfnat}\\
    & & & E_z\\
    & & & {(\sflam n {\sfprod {\alpha} \sfnat}
                                               {(\app{\app {E_s} {(\sffst n)}} {(\sfsnd n)},
                                                 {\sfs {(\sfsnd n})} )} )})\\
  \end{array}
\end{displaymath}

\section{The Compilation of System-T into System-F}\label{sec:compTtoF}

\begin{displaymath}
  \begin{array}{rcl}
    \tran \stnat & = & \sfall \alpha \alpha \to (\alpha \to \alpha) \to \alpha \\
    \tran {s \to t} & = & \tran s \to \tran t

    \vs

    \tran \cdot & = & \cdot \\
    \tran \Gamma, x\oft t & = & \tran \Gamma, x \oft \tran t

    \vs

    \tran \stz & = & \sfLam \alpha {\sflam z \alpha {\sflam f {\alpha\to\alpha} z}}\\
    \tran {\sts e} & = & \sfLam \alpha {\sflam z \alpha {\sflam f {\alpha\to\alpha} {\app f {(\app{\app {\sftapp {\tran e} {\alpha}} z} f)}}}}\\
    % \tran {\strec t e {e_z} {e_s}} & =
    %                  & \sfrec {\tran t} {\tran e} {\tran {e_z}}
    %                    {\sflam x {\sfprod {\tran t} \sfnat} (\assub {\sffst n} f {\assub{\sfsnd n}x{\tran{e_s}}})}
    % \\
    \tran {\strec t e {e_z} {e_s}} & = &
                                         \sfrec {\tran t} {\tran e} {\tran {e_z}}
                                         M
    \\
    & & \mbox{where}\\
    & & \quad M = {\sflam x {\sfprod {\tran t} \sfnat} (\assub {\sffst n} f {\assub{\sfsnd n}x{\tran{e_s}}})}\\
    \tran {\stlam x s e} & = & \sflam x {\tran s} {\tran e} \\
    \tran {\app {e_1} {e_2}} & = & \app {\tran {e_1}} {\tran {e_2}} \\
    \tran x & = & x\\
  \end{array}
\end{displaymath}

\begin{thm}[Translation Preserves Types]
  \ \\If $\mathcal{D}: \Gamma\vdash e \oft t$ then $\tran\Gamma \vdash \tran e \oft \tran t$.
\end{thm}

\begin{proof}
  \begin{flushleft}
    by structural induction on the typing derivation $\mathcal{D}$.\\

    Case: $\infer[\rl{t-z}]
      {\Gamma\vdash \stz \oft \stnat}
      {}$ \\

    $\tran\Gamma\vdash \sfz \oft \sfnat$ \hfill Given\\
    $\tran\Gamma\vdash \sfLam \alpha {\sflam z \alpha {\sflam f {\alpha\to\alpha} z}} \oft
    \sfall \alpha \alpha \to (\alpha \to \alpha) \to \alpha$ \hfill By definition\\
    Immediate application of \rl{T-tabs}, twice \rl{T-abs} and \rl{T-var}
    \vs

    Case: $\infer[\rl{t-s}]
      {\Gamma\vdash \sts e \oft \stnat}
      {\Gamma\vdash e \oft \stnat}
      $ \\
    $\tran\Gamma \vdash \tran e \oft \tran \stnat$ \hfill by i.h.\\
    $\tran\Gamma \vdash \tran e \oft \sfnat$ \hfill by translation\\
    $\tran\Gamma \vdash \sfs {\tran e} \oft \sfnat$ \hfill by \rl{T-App} and type of $\sfs{}$
    \vs

    Case: $\infer[\rl{t-rec}]
      {\Gamma\vdash \strec t e {e_z}{e_s} \oft t}
      {\Gamma\vdash e \oft \stnat
        & \Gamma\vdash e_z \oft t
        & \Gamma,f\oft t,x\oft \stnat\vdash e_s \oft t}$ \\

    $\tran\Gamma\vdash\tran e\oft \sfnat$ \hfill by i.h.\\
    $\tran\Gamma\vdash\tran{e_z}\oft \tran t$ \hfill by i.h.\\
    $\tran\Gamma,f\oft\tran t,x\oft\sfnat\vdash \tran{e_s}\oft \tran t$ \hfill by i.h.\\
    $\tran\Gamma\vdash \sfrec {\tran t} {\tran e} {\tran {e_z}}
                       {\sflam x {\sfprod {\tran t} \sfnat} (\assub {\sffst n} f {\assub{\sfsnd n}x{\tran{e_s}}})}$\\
                       \hfill by simple typing derivation
   \vs

    Case: $\infer[\rl{t-abs}]
      {\Gamma\vdash \stlam x s e \oft s \to t}
      {\Gamma, x \oft s\vdash e \oft t}
      $ \\
    $\tran\Gamma,x\oft\tran s \vdash \tran e \oft \tran t$ \hfill by i.h.\\
    $\tran\Gamma\vdash \sflam x {\tran s} {\tran e}$ \hfill by \rl{T-lam}
    \vs

    Case: $\infer[\rl{t-app}]
      {\Gamma\vdash \app{e_1}{e_2} \oft t}
      {\Gamma\vdash e_1\oft s \to t
        & \Gamma \vdash e_2 \oft s}$ \\

    $\tran\Gamma\vdash \tran{e_1} \oft \tran s \to \tran t$ \hfill by i.h.\\
    $\tran\Gamma\vdash \tran{e_2} \oft \tran s$ \hfill by i.h.\\
    $\tran\Gamma\vdash \app {\tran{e_1}} {\tran{e_2}} \oft \tran t$ \hfill by \rl{T-app}
    \vs

    Case: $\infer[\rl{t-var}]
      {\Gamma \vdash x \oft t}
      {x\oft t \in \Gamma}$\\

    $x\oft t \in \Gamma$ \hfill given\\
    $x\oft \tran t \in \tran\Gamma$ \hfill by property of translation of contexts\\
    $\tran\Gamma\vdash x \oft \tran t$ \hfill by \rl{T-var}
  \end{flushleft}
\end{proof}

%% Local Variables:
%% mode: latex
%% TeX-master: "../thesis"
%% End:
